# Supplementary material for: Personalized Instance-based Navigation Toward User-Specific Objects in Realistic Environments
Source: arXiv:2410.18195 source file (2025-02-19)
Supplement: Supplementary file 1 [file sizes.tex]

\begin{table}[!t]
  \centering
  \caption{Ratio of the part of the sample images depicting each target object category in comparison with the area of the full image and the percentage of activations of the open-set object detector. 
  The perthousand object/image ratio is computed using both the segmentation mask and the bounding box of each target objects. The activation ratio of the object detector is instead computed as a percentage.
  }
  \label{tab:size_in_image}
  \resizebox{\linewidth}{!}{
  \begin{tabular}{lC{1.5cm}C{1.5cm}C{1.5cm} c lC{1.5cm}C{1.5cm}C{1.5cm}}
    \toprule
    Category & \textperthousand SegMask & \textperthousand BBox & \%Act & & Category & \textperthousand SegMask & \textperthousand BBox & \%Act \\
    \midrule
    \textbf{Backpack} & 12.76 & 16.56 & 48.55 && \textbf{Keys} & 0.16 & 0.34 & 0.17 \\
    \rowcolor{light_gray} 
    \textbf{Bag} & 8.10 & 12.81 & 47.26 && \textbf{Laptop} & 7.20 & 12.25 & 56.84 \\
    \textbf{Ball} & 4.54 & 5.96 & 33.33 && \textbf{Mug} & 1.28 & 1.54 & 1.33 \\
    \rowcolor{light_gray} 
    \textbf{Book} & 3.73 & 5.06 & 16.03 && \textbf{Shoes} & 3.49 & 5.53 & 19.35\\
    \textbf{Camera} & 1.99 & 2.59 & 4.76 && \textbf{Teddy Bear} & 12.36 & 20.78 & 78.85 \\
    \rowcolor{light_gray} 
    \textbf{Cellphone} & 0.75 & 0.80 & 1.28 && \textbf{Toy} & 4.30 & 9.68 & 13.78 \\
    \textbf{Eyeglasses} & 0.49 & 1.22 & 3.69 && \textbf{Visor} & 2.71 & 4.57 & 0.64 \\
    \rowcolor{light_gray} 
    \textbf{Hat} & 3.34 & 5.97 & 11.60 && \textbf{Wallet} & 0.85 & 1.05 & 2.05 \\
    \textbf{Headphones} & 3.36 & 5.84 & 11.72 && \textbf{Watch} & 0.30 & 0.52 & 0.80 \\
    \bottomrule
  \end{tabular}
  }
\end{table}
